# Supplementary material for: HOComp: Interaction-Aware Human-Object Composition
Source: arXiv:2507.16813 source file (2025-07-22)

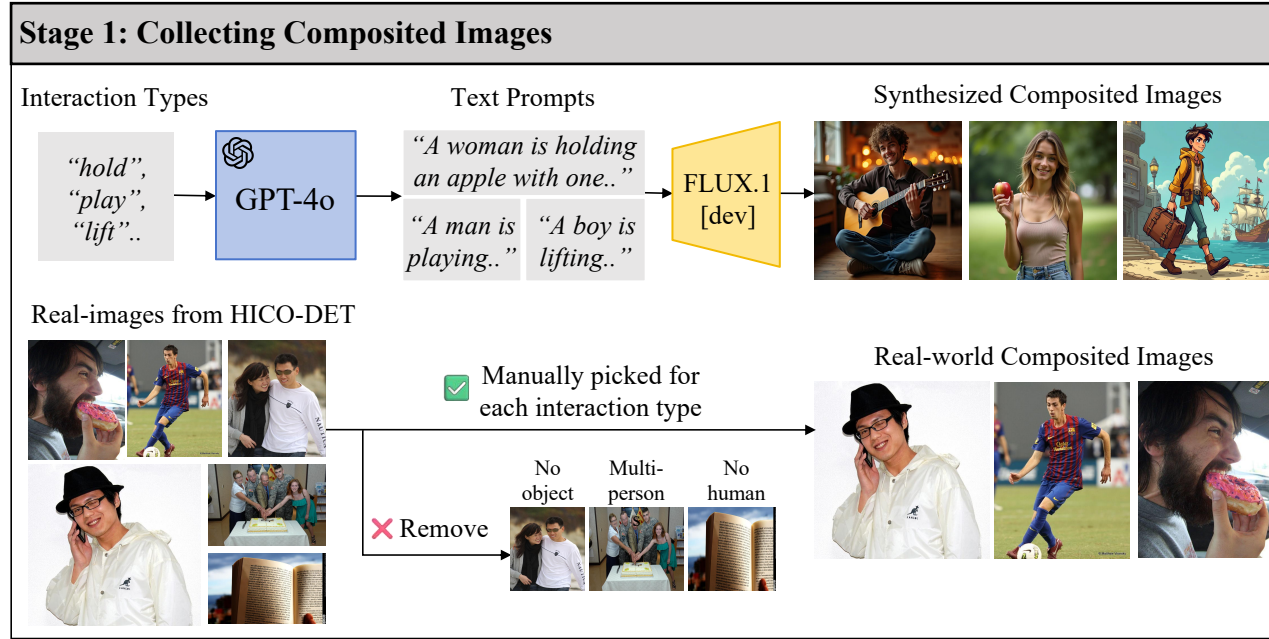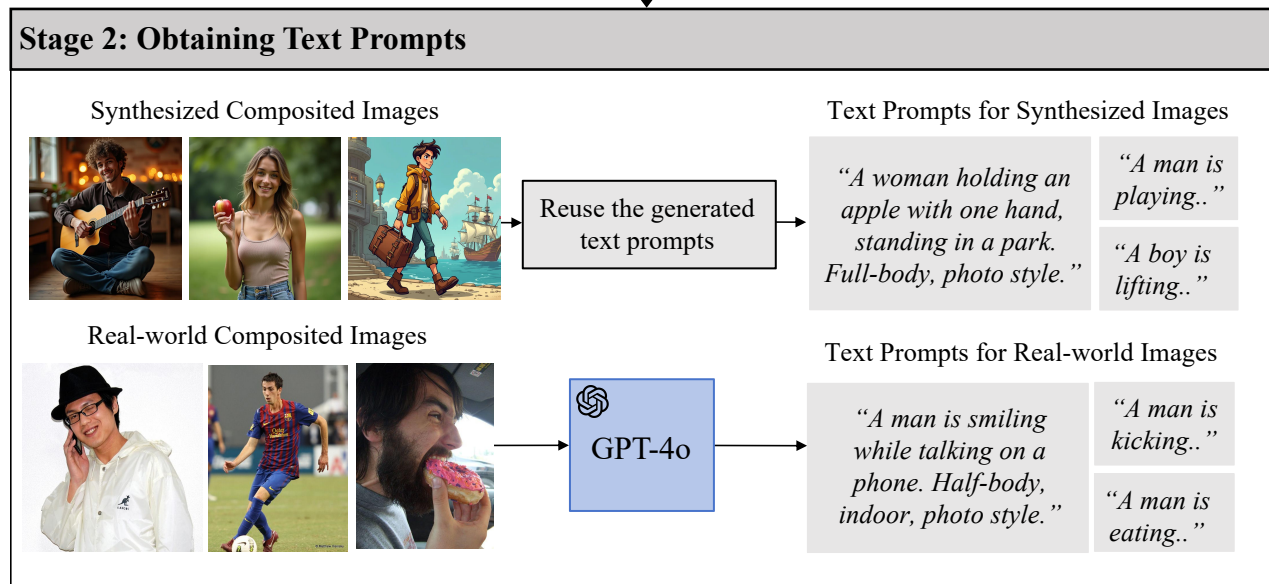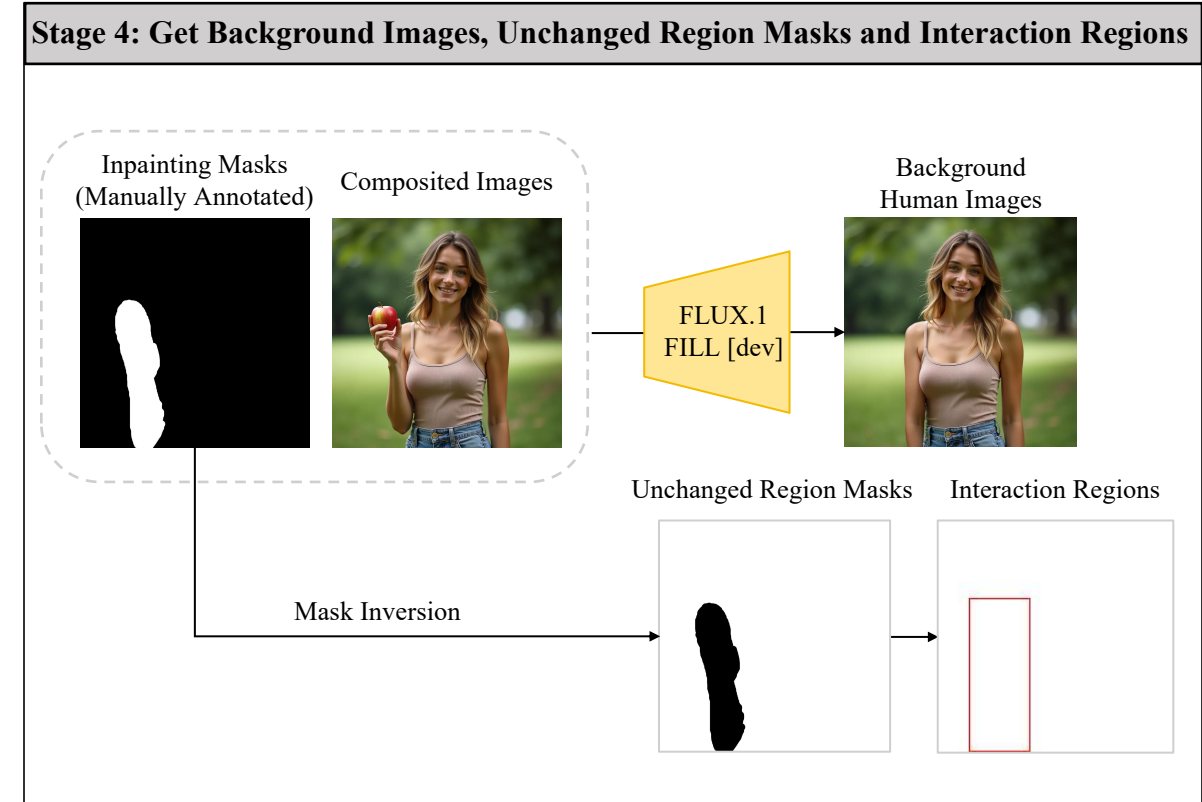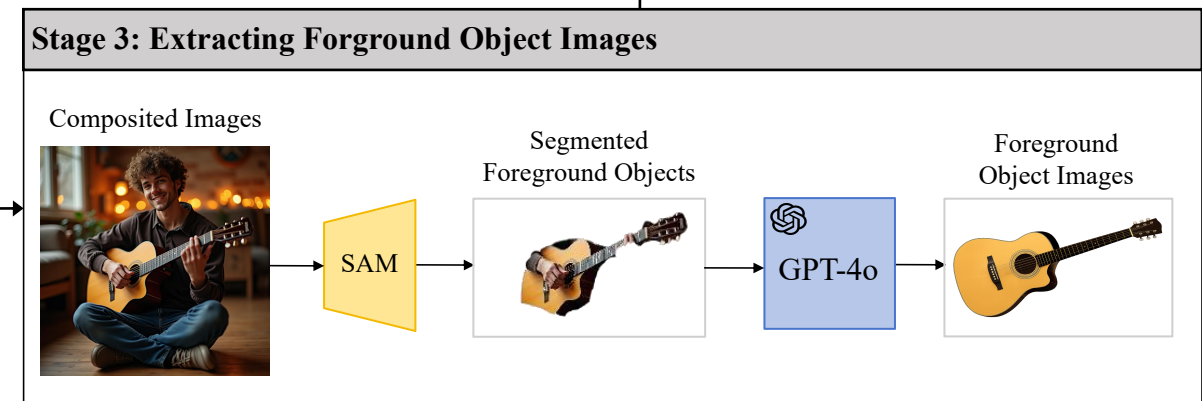



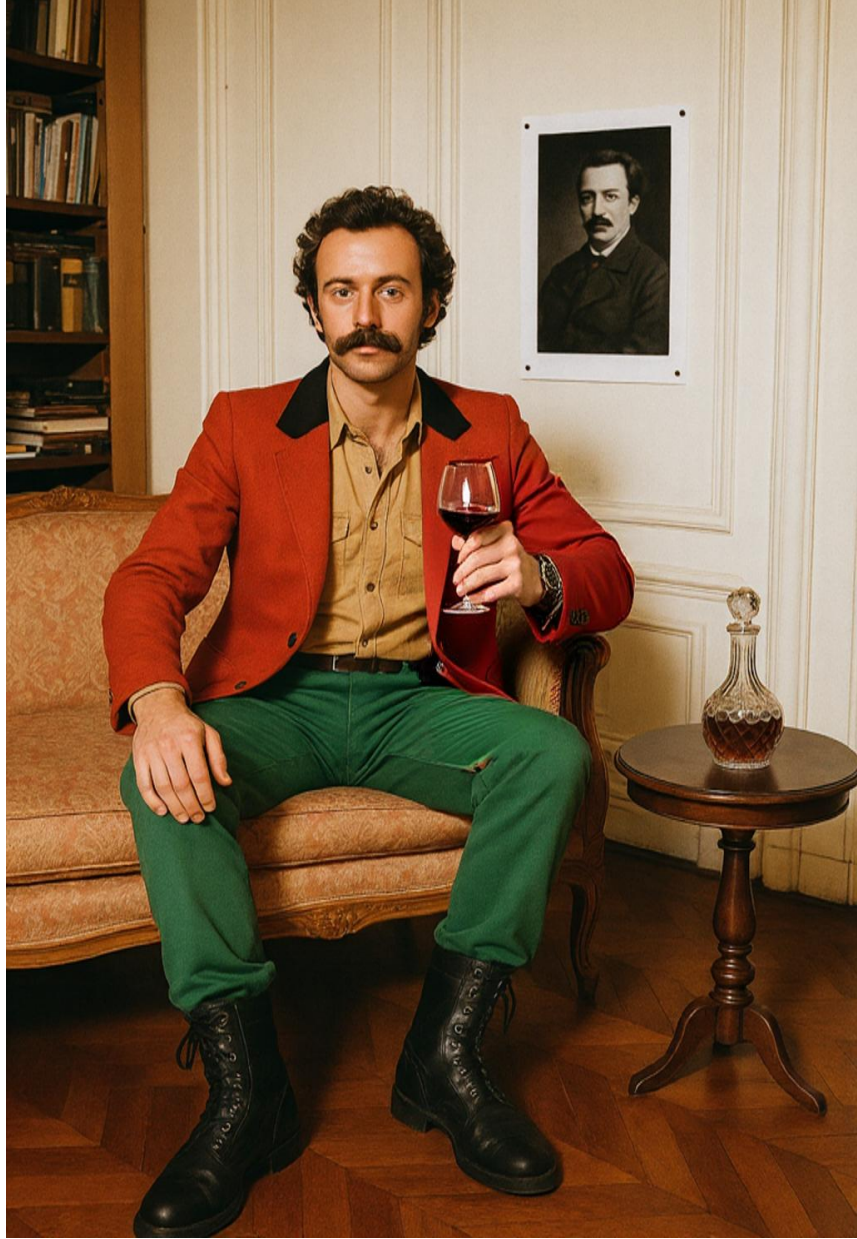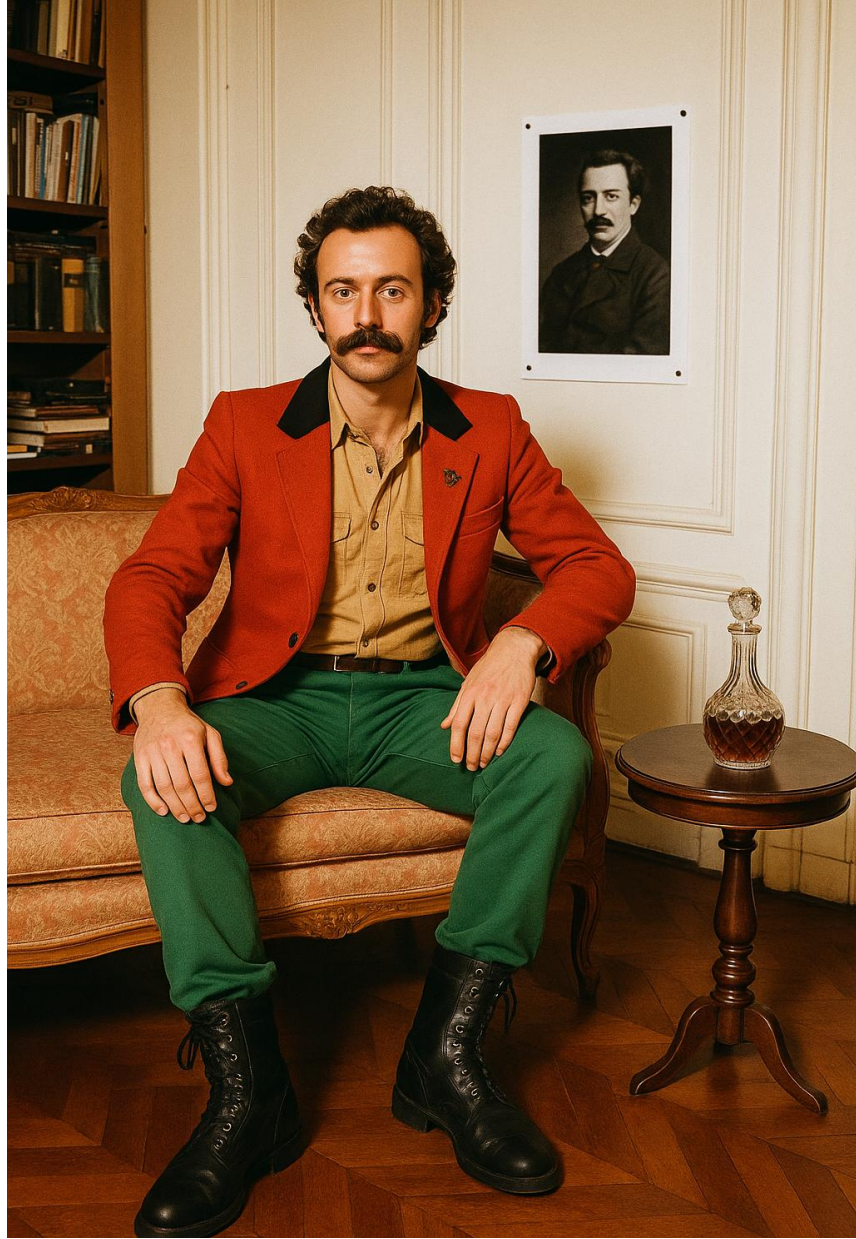

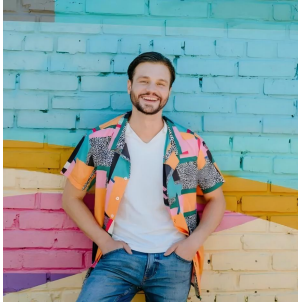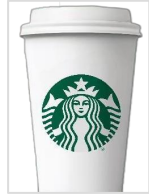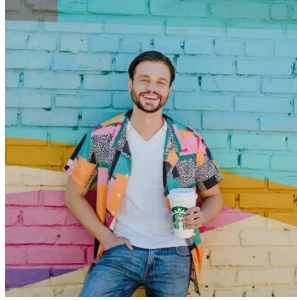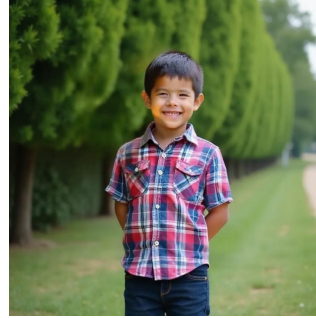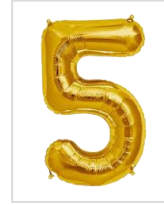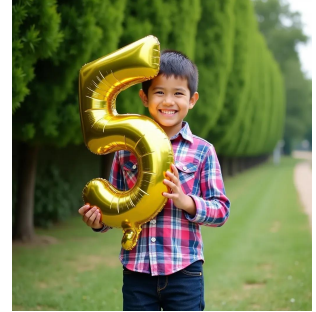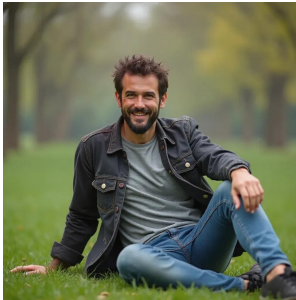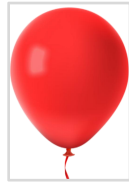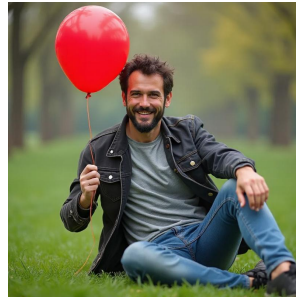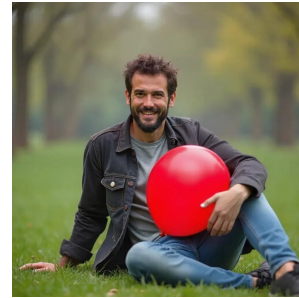



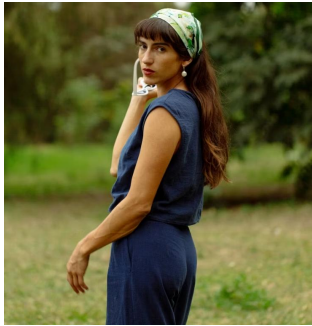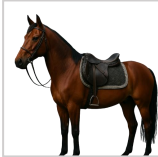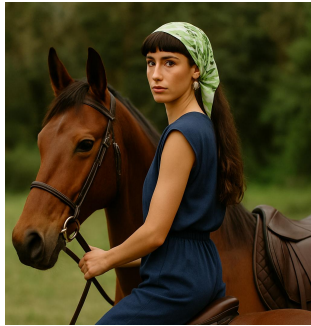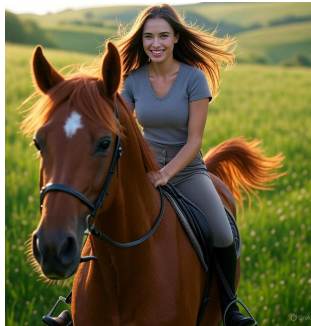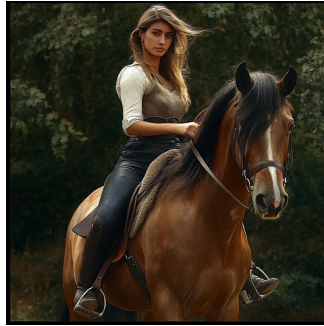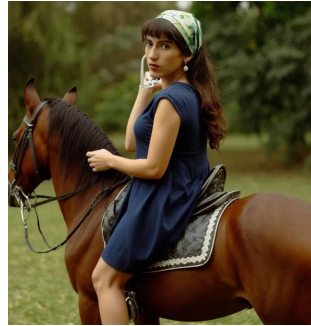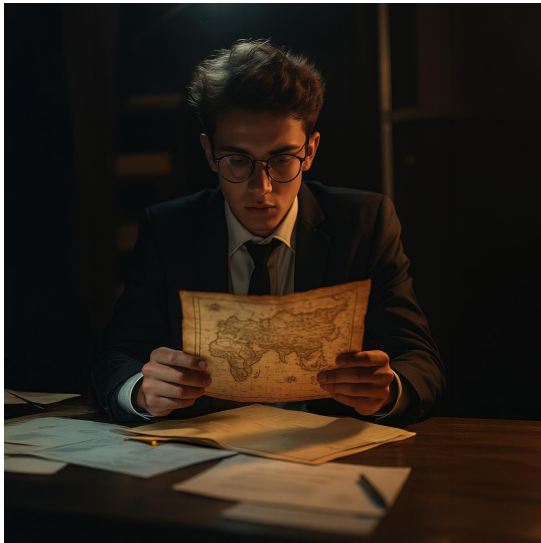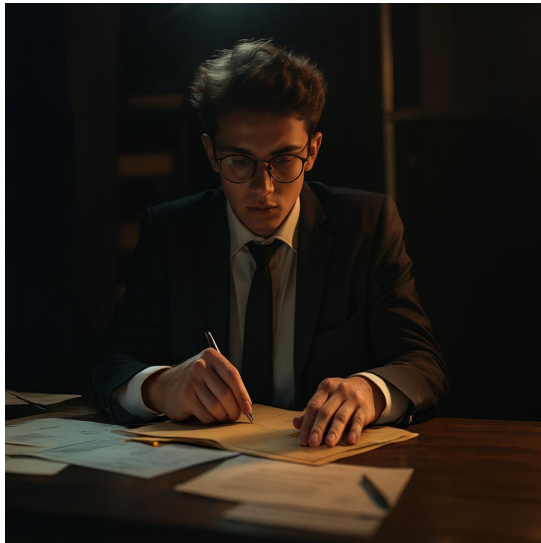

Supplement: Supplementary file 1 [file dataset_construct.pdf]
